# Supplementary material for: KUDA: Keypoints to Unify Dynamics Learning and Visual Prompting for Open-Vocabulary Robotic Manipulation
Source: arXiv:2503.10546 source file (2025-03-13)
Supplement: Supplementary file 1 [file 6_appendix.tex]

% concerns:
% 1. error breakdown
% 2. dynamics model, keypoint specification, VLM feedback
% 3. generalization (both prompt and dynamics model)

\section*{APPENDIX \\IMPLEMENTATION DETAILS} \label{app:1}

% Method:
%     1. pseudocode
%     2. implement of our dynamics model
%     3. keypoint specification:
%         1. how we get the keypoints
%         2. how we annotate
%         3. text prompt and annotated image example
%         4. how we get keypoint specification from the response
%     4. top-k library, how we pick top-k examples
%     5. dynamics planning and closed-loop control:
%         1. how we use MPPI
%         2. how to use tracking for low-level closed-loop
%         3. high-level closed-loop

The pseudocode of our method is Algo \ref{algo:1}, and the implementation details of each component are in the following sections.

\begin{algorithm}[htbp]
    \caption{KUDA}
    \label{algo:1}
    \begin{algorithmic}[1]
        \Require Vision-language Model $\mathcal{M}$, Dynamics Model $f$, Prompt Retriever $\mathcal{R}$, Point Tracker $\mathcal{T}$, Language Instruction $\mathcal{L}$, Text Prompt $p_\text{base}$, Prompt Library $\mathcal{P} = \{(q_i, \text{obs}_i, r_i)\}$
        \For{high-level iteration $r = 0, \dots, N - 1$}
            \State Get observation $s_0$, environment state $z_0$ from the top down camera
            \State Propose keypoints and get the annotated image $A(s_0)$, use retriever $\mathcal{R}$ to get the top-k examples $\mathcal{R}(\{(q_i, \text{obs}_i, r_i)\})$
            \State Prompt the VLM to obtain the target specifications $\text{TS} = \mathcal{M}(p_\text{base}, A(s_0), \mathcal{R}(\{(q_i, \text{obs}_i, r_i)\}))$
            \For{low-level iteration $t = 0, \dots, \text{n\_actions} - 1$}
                \State Obtain objective $\mathcal{C}(z|\mathcal{L}) = \sum_{i\in\text{TS}}\sqrt{(o_i - p_i)^2}$ from target specifications.
                \State Optimize $\mathcal{C}(z|\mathcal{L})$ with $f$ to get the action $a_t$
                \State Execute $a_t$ on the robot
                \State Obtain environment state $z_{t + 1}$ and use tracking module $\mathcal{T}$ to update target specifications.
            \EndFor
        \EndFor
    \end{algorithmic}
\end{algorithm}

\subsection{Dynamics Models} \label{app:1.1}

We utilize two types of neural dynamics models: the graph-based neural dynamics model and the state-based neural dynamics model. The graph-based model follows the framework presented in \cite{li2018learning}. Specifically, an object is represented as a graph with vertices $O = \{o_i\}$, where each vertex represents a particle, and edges $R = \{r_k\}$, which capture the relationships between particles. Each vertex $o_i$ is defined as $o_i = \langle x_i, a_i^o \rangle$, where $x_i = \langle q_i, \dot{q}_i \rangle$ represents the state of particle $i$ (including its position $q_i$ and velocity $\dot{q}_i$), and $a_i^o$ denotes its attributes. Each edge $r_k$ is defined as $r_k = \langle u_k, v_k, a_k^r \rangle$, where $u_k$ and $v_k$ denote the receiver and sender vertices, respectively, and $a_k^r$ represents the type and attributes of the relationship.

At each time step $t$, we employ two encoders, $f_O^\text{enc}$ and $f_R^\text{enc}$, to compute latent embeddings for the vertices and edges, respectively:
\begin{equation}
    h_{o_i, t}^0 = f_O^\text{enc}(o_{i, t}),\quad h_{r_k, t}^0 = f_R^\text{enc}(r_{k, t}).
\end{equation}

Next, an edge propagation network $f_R^\text{prop}$ and a vertex propagation network $f_O^\text{prop}$ are used to iteratively update the embeddings of edges and vertices through multi-step message passing. For $l = 0, 1, \dots, L - 1$, the updates are computed as:
\begin{align}
    h_{r_k, t}^{l + 1} &= f_R^\text{prop}(h_{u_k, t}^l, h_{v_k, t}^l), \\
    h_{o_i, t}^{l + 1} &= f_O^\text{prop}\left(h_{o_i, t}^l, \sum_{j \in \mathcal{N}(o_{i, t})} h_{r_k, t}^{l + 1}\right).
\end{align}
where $\mathcal{N}(o_{i, t})$ denotes the set of edge indices where vertex $i$ acts as the receiver at time $t$, and $L$ is the total number of message passing steps.

Finally, a vertex decoder $f_O^\text{dec}$ is employed to predict the state of the object at the next time step, given the updated vertex embedding:
\begin{equation}
    \hat{o}_{i, t+1} = f_O^\text{dec}(h_{o_i, t}^L).
\end{equation}

To construct the graph $\{O, R\}$ in our approach, we utilize a top-down RGB-D camera to capture observations and utilize GroundingSAM~\cite{ren2024grounded} to segment objects and extract their corresponding point clouds. The farthest point sampling method is then applied with a fixed pointwise distance threshold $r$ to generate particles representing the objects. For the two types of pushers used in our study, we represent the cylinder stick with a single particle and the board pusher with five particles. Edges between particles are established based on a spatial distance threshold $d$. In our implementation, we set $r = 0.02 \ \text{m}$ and $d = 0.06 \ \text{m}$.

% To construct the graph $\{O, R\}$ in our work, we use a top-down RGB-D camera to capture the observation and GroundingSAM~\cite{ren2024grounded} to segment the object and obtain the object’s point cloud. We then apply the farthest point sampling method with a fixed pointwise distance threshold $r$ to generate the object particles. For the two types of pushers used in our study, we represent the cylinder stick with one particle and the board pusher with five particles. Edges between all particles are constructed based on a spatial distance threshold $d$. In our work, we set $r = 0.02 \text{m}$ and $d = 0.06 \text{m}$.

The data generation for our graph-based dynamics model training is achieved by NVIDIA FleX~\cite{li2018learning, macklin2014unified}, a position-based simulation framework tailored for modeling interactions involving various materials, including deformable objects. For each material, we collected a dataset comprising 1000 episodes, where each episode includes 5 randomly generated robot-object interactions. For the rope material, we randomize the length and stiffness of the rope, and for the granular material, we randomize the granular size, to enable our model to handle objects with different physical parameters. (You can see this in our demo, we used different kinds of rope and granular pieces.) To improve robustness during training, we incorporated rotational randomness into the simulation. Furthermore, our model is designed to be translation-equivariant, relying solely on velocity and position difference information within the network.

% The data generation for our graph-based dynamics models is conducted using NVIDIA FleX~\cite{li2018learning, macklin2014unified}, a position-based simulation framework specifically designed for modeling interactions between various materials, including deformable objects. For each material, we collected 1000 episodes, with each episode comprising 5 random robot-object interactions. To enhance robustness during training, we introduced rotational randomness, and our model is designed to be translation-equivariant (we will only utilize velocity and position difference information in our network).

% The data generation for our graph-based dynamics models is performed in NVIDIA FleX~\cite{li2018learning, 10.1145/2601097.2601152}, a position-based simulation framework designed for modeling interactions between different materials including deformable objects. For each material we collected 1000 episodes with each episode contains 5 random robot-object interactions. During training we add rotation randomness for robustness, and our model is designed to be translation equivariant.

For T-shaped block in our work, we use four keypoints' x, y positions to represent T's state, which contains the top center point $tc$, top right point $tr$, top left point $tl$, and bottom center point $bt$ when T is upright. At time $t$, the state-based neural network receives $(tc_t, tr_t, tl_t, bt_t, p_t, a)$ as input, where $p_t$ is the current pusher position, and $a$ represents the action of the pusher. Then the network will predict $(tc_{t + 1}, tr_{t + 1}, tl_{t + 1}, bt_{t + 1}, p_{t + 1})$ for the next time step.

To obtain the keypoints of the T-shaped block in the real world, we first use the same pipeline as in the graph-based neural dynamics model to extract the point cloud of the T-shaped block. We then apply the Iterative Closest Point (ICP) algorithm~\cite{924423} to estimate the block's 6D pose and calculate the positions of its keypoints. The T-shaped block used in our experiments measures 12 cm in height and 12 cm in width, with both the stem and bar having a width of 3 cm.

In our experiments, we employ different end effectors tailored to specific task requirements. The board pusher, used for manipulating cubes and granular pieces, has dimensions of 10 cm $\times$ 0.5 cm on the horizontal plane, whereas the cylinder pusher, designed for interacting with ropes and T-shaped objects, has a diameter of 1 cm.

The data generation for our state-based dynamics model is performed using Pymunk~\cite{pymunk}, a 2D physics library for simulating rigid body dynamics. For the T-shaped block, we collected a dataset of 20,000 episodes, with each episode consisting of 300 random robot-object interactions. During both training and inference, all coordinates are transformed into the block's local coordinate system, making our model both translation-equivariant and rotation-equivariant.

% To obtain the keypoints in the real world for the T-shaped block, we first use the same pipeline as in the graph-based neural dynamics to get the point cloud of T, then we use the ICP algorithm~\cite{924423} to get T's 6D pose, and calculate the keypoints' positions of T. The T-shaped block used in our experiment is 12cm in height and 12cm in width, with the stem and bar being 3cm in width.

% The data generation for our state-based dynamics model is conducted in Pymunk~\cite{pymunk}. Pymunk is a 2d physics library that can be used for rigid body physics. We collected 20000 episodes for T-shaped block, each contains 300 random robot-object interactions. We transform all coordinates into T's own coordinate system when training and inferring, so our model is translation-equivariant and rotation-equivariant.

All training processes are performed on a Linux machine equipped with a CPU of 32 cores and 2 NVIDIA RTX 4090 GPUs.

\subsection{Target Specification} \label{app:1.2}

% We demonstrate the implementation details in Section \ref{sec:3.2} here. After obtaining the RGB image from the top-down camera, we use SAM~\cite{kirillov2023segment} to generate all the semantic masks. The mask with the largest area, typically representing the background, is removed. We then apply the farthest point sampling method with a fixed pointwise radius threshold to extract up to eight keypoints for each mask. Additionally, the center of each mask is included as a keypoint, as it is often geometrically representative.

% Next, the farthest point sampling method is applied with a global radius threshold to all keypoints to prevent an excessive concentration of keypoints at the edges. For each keypoint, a red dot is annotated on the original image, along with an assigned index placed above the red dot. A green dot is also annotated at the center of the image, labeled as 'C', to serve as a reference point if no other objects are present on the table.

% The implementation details are provided in Section \ref{sec:3.2}.

We demonstrate the implementation details in Section~\ref{sec:3.2} here. After capturing an RGB image using the top-down camera, we utilize SAM~\cite{kirillov2023segment} to generate semantic masks for all objects in the scene. The mask with the largest area, which typically corresponds to the background, is discarded. For each remaining mask, we apply the farthest point sampling method with a fixed pointwise radius threshold to extract up to eight keypoints. Additionally, the center of each mask is included as a keypoint, as it often serves as a geometrically representative feature.

Subsequently, we apply the farthest point sampling method again, this time with a global radius threshold across all keypoints, to prevent excessive clustering near the edges. Each keypoint is marked on the original image as a red dot, with its index displayed above the dot. Additionally, a green dot is annotated at the center of the image and labeled as `C', serving as a reference point when no other objects are present on the table.

All annotated points include both the keypoints on the objects and the reference points in the environment; they are not distinguished during annotation, as the VLM can typically recognize which points correspond to objects. We provide the example of our text prompt to the VLM in~\ref{lst:1}. Please see more detailed annotated image examples and text prompts in our code repository. We ensure that examples in the prompt library do not duplicate the objects and the instructions in evaluation tasks.

\lstset{
    basicstyle=\ttfamily\footnotesize,
    backgroundcolor=\color{gray!9},
    frame=single,
    breaklines=true,
}

\subsection{Dynamics Planning and Two Level Closed-loop Control} \label{app:1.3}

After projecting the target specifications into 3D space, as described in \nameref{app:1.2}, and obtaining the cost function, we apply the MPPI algorithm~\cite{williams2015model} to determine the next action. Specifically, starting from the initial environment state $z_0$, we iteratively sample actions $\{a_i\}_{i = 0}^T$ from the action space, where $T$ represents the look-ahead horizon. The dynamics model is then used to predict the outcome of each trajectory. Using the cost function, we calculate the weight of each trajectory and synthesize these trajectories to derive the final action sequence ${a_i}$ that minimizes the cost function. In our setup, each action is a push along a straight line, with the starting point within the workspace and a length of no more than 20 cm.

% After we project the target specifications into 3D space as described in \nameref{app:1.2} and obtain the cost function, we then apply MPPI~\cite{williams2015model} to get the next action. To be more specific, from each start environment state $z_0$, we iteratively sample actions $\{a_i\}_{i = 0}^T$ from the action space, where $T$ is the look-ahead horizon, and apply the dynamics model to predict the outcome for each trajectory. And then, we use the cost function to calculate the weight of each trajectory, and synthesis these trajetories to get the final result $\{a_i\}$ that minimize the cost function. In our work, each action is a push along a straight line, with the starting point in the workspace and length being shorter than 20cm.

To achieve closed-loop control at the dynamics planning level, we record a video of each action using a side camera. We then input all object particles, including keypoints from the target specifications, along with the recorded video into SpatialTracker~\cite{xiao2024spatialtracker} to obtain the positions of the tracked particles after each action. However, we observed that the tracked particles exhibit some errors, similar to the prediction errors from the dynamics model, making them unsuitable for the next optimization iteration. To address this, we update the target specifications by resampling the particles from the objects after each action. The tracked keypoints are then calibrated to their nearest neighbors among the newly sampled particles, and the target specifications and cost function are updated accordingly. Our experiment results demonstrate that this method effectively preserves the stability of the cost function.

% To achieve the dynamics planning level closed-loop, during each action we use a side camera to record a video. Then we input all the object particles (include keypoints in target specifications) and recorded video to SpatialTracker~\cite{xiao2024spatialtracker} to get the tracking particles' positions after each action. However, we found that these tracking particles also have some errors just like the prediction result from the dynamics model, and are not compatible for the next iteration of optimizing, so we choose to update the target specifications: after each action we sample the particles from the objects again, and calibrate those tracking keypoints to their nearest neighbors in the particles, and update the target specifications and the cost function. Experiments show that this method can maintain the stability of the cost function well.

To achieve closed-loop control at the VLM level, after a certain number of actions, we terminate the optimization process and update the current observation along with the language instruction to prompt the VLM in the next loop, generating a new target specification. Experimental results indicate that this method is particularly effective in under-specified tasks, where the number of keypoints is insufficient to accurately define a target for the objects. Additionally, it helps correct instances where the VLM provides incorrect target specifications.

% To achieve the VLM level closed-loop, after a number of actions has been applied, we will terminate the optimization process, and use current observation with the language instruction to prompt the VLM again, and obtain a new target specification. Experiments show that this method is effective in some under-specific tasks, i.e. the number of keypoints is too small to specify a good target for the objects, and it can correct some cases where the VLM gives incorrect target specifications.

% \subsection{Discussions on Error Breakdown} \label{app:1.4}

% In our experiment setup, we use a top-down camera to capture the images as the input for the large vision model and visual prompting for the vision language model. During robot execution for model-based planning, we use the side camera to track keypoints. However, there are occlusions caused by the robot arms or end-effectors, especially for small granular objects like coffee beans. \Mingtong{Please explain different cases}.
